# Supplementary material for: Out-of-Distribution Detection for LiDAR-based 3D Object Detection
Source: arXiv:2209.14435 source file (2022-09-28)
Supplement: Supplementary file 1 [file X_supplementary.tex]

\appendix

% --- PDF will be split by an editor (e.g. macOS preview), so need to restart
% from page 1
\setcounter{page}{1}

% --- repeat the title (AT: haven't found a more elegant way to do this...)
\twocolumn[
\centering
\Large \textbf{Supplementary Material} \\
\vspace{1.0em}
] %< twocolumn
\appendix
\section{Evaluation metrics}
% \EndIf
\textbf{AUROC} is the measure of the area under the plot of true positive rate
(TPR) vs. false positive rate (FPR). It measures the probability that an OOD
example is assigned a lower score than an ID example. TPR is computed as
$\mathrm{TPR}=\mathrm{TP}/(\mathrm{TP} + \mathrm{FN})$ and FPR is computed as
$\mathrm{FPR}=\mathrm{FP}/(\mathrm{FP}+\mathrm{TN})$, where TP, FP, TN, and FN
denote True Positive, False Positive, True Negative, and False Negative,
respectively.

\textbf{AUPR} is the Area under the Precision-Recall curve. The PR curve is a
graph showing the $precision=\mathrm{TP}/(\mathrm{TP}+\mathrm{FP})$ and
$recall=\mathrm{TP}/(\mathrm{TP}+\mathrm{FN})$ against each other. The metric
AUPR-In and AUPR-Out are the area under the precision-recall curve where ID and
OOD samples are specified as positives, respectively.

\textbf{Detection Error} $D_e$ measures the misclassification probability when
TPR is 95\%. The formula to calculate $D_e = 0.5(1 - \mathrm{TPR}) +
0.5\mathrm{FPR} $, where we assume that both positive and negative examples have
equal probability of appearing in the test set.

\textbf{FPR @ 95\% TPR} is the probability that an OOD (negative) example is
correctly identified when the TPR is 95\%.  
\section{Additional results}
% We present full results of our experiments on different layers and OOD
% datasets. The results show that all methods do relatively well in the
% contrastive layer for KITTI Ignored objects. Especially, OCSVM has a huge
% boost in performance. The best performing model in Waymo objects is
% normalizing flows with conv4x features.
\begin{table*}
\centering
\tiny
\begin{tabular}{rc|ccc|ccc|ccc|ccc|ccc}
\toprule
        &       & \multicolumn{3}{c}{AUROC} & \multicolumn{3}{c}{AUPR (ID)} & \multicolumn{3}{c}{AUPR (OOD)} & \multicolumn{3}{c}{FPR @ 95\% TPR} & \multicolumn{3}{c}{Detection Err.} \\
       \textbf{OOD Method} &    \textbf{Layer}   &   Base &  Ctrst & $\Delta$ &      Base &  Ctrst & $\Delta$ &       Base &  Ctrst & $\Delta$ &           Base &  Ctrst & $\Delta$ &           Base &  Ctrst & $\Delta$ \\
\midrule
\textbf{Max Softmax} & \textbf{-} &  89.95 &  \underline{\textbf{89.97}} &     \textbf{0.02} &     91.46 &  \underline{\textbf{91.85}} &     \textbf{0.38} &      \underline{\textbf{88.01}} &  \underline{\textbf{87.66}} &    -0.35 &          33.83 &  \underline{\textbf{31.86}} &    \textbf{-1.97} &          19.33 &  \underline{\textbf{18.32}} &    \textbf{-1.00} \\
\textbf{Predictive Entropy} & \textbf{-} &  83.49 &  84.80 &     \textbf{1.32} &     87.50 &  88.94 &     \textbf{1.44} &      76.48 &  77.56 &     \textbf{1.08} &          39.60 &  34.54 &    \textbf{-5.05} &          22.19 &  19.65 &    \textbf{-2.54} \\
\textbf{Aleatoric Entropy} & \textbf{-} &  83.09 &  84.65 &     \textbf{1.56} &     87.03 &  88.67 &     \textbf{1.64} &      75.93 &  77.75 &     \textbf{1.82} &          41.77 &  36.41 &    \textbf{-5.37} &          23.29 &  20.57 &    \textbf{-2.71} \\
\textbf{Mutual Information} & \textbf{-} &  60.48 &  60.70 &     \textbf{0.23} &     54.10 &  54.79 &     \textbf{0.69} &      64.48 &  63.87 &    -0.61 &          97.07 &  96.51 &    \textbf{-0.56} &          49.98 &  49.83 &    \textbf{-0.15} \\
\midrule
\multirow{6}{*}{\textbf{Mahalanobis}} & \textbf{logits} &  66.55 &  67.76 &     \textbf{1.21} &     59.28 &  59.04 &    -0.25 &      71.47 &  72.36 &     \textbf{0.88} &          93.81 &  95.31 &     1.51 &          49.16 &  49.70 &     0.54 \\
        & \textbf{backbone} &  \textbf{83.77} &  \textbf{84.56} &     \textbf{0.80} &     \textbf{85.30} &  \textbf{86.73} &     \textbf{1.43} &      \textbf{81.65} &  \textbf{81.93} &     \textbf{0.28} &          \textbf{51.01} &  \textbf{43.92} &   \textbf{-7.10} &          \textbf{27.89} &  \textbf{24.34} &    \textbf{-3.55} \\
        & \textbf{conv2x} &  79.37 &  79.48 &     \textbf{0.11} &     78.46 &  77.89 &    -0.56 &      77.93 &  78.78 &     \textbf{0.85} &          70.36 &  72.44 &     2.07 &          37.55 &  38.55 &     1.00 \\
        & \textbf{conv4x} &  66.94 &  69.12 &     \textbf{2.18} &     64.28 &  66.95 &     \textbf{2.67} &      66.12 &  67.91 &     \textbf{1.79} &          87.43 &  83.99 &    \textbf{-3.44} &          46.11 &  44.41 &    \textbf{-1.70} \\
        & \textbf{conv8x} &  62.71 &  68.68 &     \textbf{5.97} &     60.76 &  69.02 &     \textbf{8.26} &      59.53 &  64.91 &     \textbf{5.38} &          90.34 &  79.83 &   \textbf{-10.51} &          47.55 &  42.32 &   \textbf{-5.23} \\
        & \textbf{ctrst} &    - &  74.89 &      - &       - &  68.37 &      - &        - &  76.07 &      - &            - &  87.09 &      - &            - &  45.91 &      - \\
\midrule
\multirow{5}{*}{\textbf{OCSVM}} & \textbf{logits} &  52.53 &  46.45 &    -6.08 &     51.69 &  45.98 &    -5.71 &      57.43 &  54.11 &    -3.32 &          93.75 &  97.78 &     4.03 &          48.16 &  49.96 &     1.79 \\
        & \textbf{conv2x} &  60.28 &  61.47 &     \textbf{1.19} &     68.82 &  69.42 &     \textbf{0.60} &      75.62 &  75.94 &     \textbf{0.32} &          79.80 &  80.28 &     0.48 &          42.25 &  42.53 &     0.28 \\
        & \textbf{conv4x} &  51.38 &  52.51 &     \textbf{1.13} &     49.92 &  50.93 &     \textbf{1.02} &      70.07 &  70.58 &     \textbf{0.51} &          97.95 &  97.94 &    \textbf{-0.01} &          49.97 &  49.95 &    \textbf{-0.02} \\
        & \textbf{conv8x} &  \textbf{65.44} &  \textbf{62.91} &    -2.53 &    \textbf{ 78.76} &  \textbf{79.93} &     \textbf{1.17} &      \textbf{78.83} &  \textbf{78.54} &    -0.29 &         \textbf{ 66.20} &  \textbf{70.31} &     4.11 &          \textbf{35.31} &  \textbf{37.17} &     1.86 \\
        & \textbf{ctrst} &    - &  58.58 &      - &       - &  49.88 &      - &        - &  70.75 &      - &            - &  98.15 &      - &            - &  49.99 &      - \\
\midrule
\multirow{6}{*}{\textbf{RealNVP}} & \textbf{logits} &  63.84 &  61.46 &    -2.38 &     61.93 &  60.33 &    -1.59 &      63.24 &  60.20 &    -3.04 &          88.02 &  89.11 &     1.09 &          46.38 &  46.83 &     0.46 \\
        & \textbf{backbone} & \underline{\textbf{90.28}}&  88.30 &    -1.98 &     \underline{\textbf{92.67}} &  \textbf{90.89} &    -1.78 &     \textbf{ 86.93} &  \textbf{84.72} &    -2.21 &         \underline{\textbf{26.72}} &  33.14 &     6.42 &          \underline{\textbf{15.72}} &  18.97 &     3.25 \\
        & \textbf{conv2x} &  78.09 &  83.64 &     \textbf{5.56} &     76.87 &  84.42 &     \textbf{7.56} &      78.58 &  81.57 &     \textbf{2.99} &          66.04 &  51.86 &   \textbf{-14.18} &          35.34 &  28.33 &    \textbf{-7.01} \\
        & \textbf{conv4x} &  87.56 &  \textbf{88.41} &     \textbf{0.85} &     88.52 &  89.66 &     \textbf{1.15} &      86.61 &  86.27 &    -0.33 &          48.26 &  41.69 &    \textbf{-6.57} &          26.52 &  23.16 &    \textbf{-3.36} \\
        & \textbf{ctrst} &    - &  87.32 &      - &       - &  89.38 &      - &        - &  83.19 &      - &            - &  \textbf{32.95} &      - &            - &  \textbf{18.89} &      - \\
\bottomrule
\end{tabular}
\caption{Results for all common OOD objects detected by both base and contrastive models. For Mahalanobis distance, OC-SVM, and RealNVP, we bold the best performing layer for each method. The best performing OOD method/layer for each metric is underlined. We also report the difference $\Delta$ between contrastive model and base model, with bold numbers indicating contrastive model has better performance. All results are averaged over three sets of experiments.}
\label{tab:full_results_all}
\end{table*}

\begin{table*}
\centering
\tiny
\begin{tabular}{rc|ccc|ccc|ccc|ccc|ccc}
\toprule
        &       & \multicolumn{3}{c}{AUROC} & \multicolumn{3}{c}{AUPR (ID)} & \multicolumn{3}{c}{AUPR (OOD)} & \multicolumn{3}{c}{FPR @ 95\% TPR} & \multicolumn{3}{c}{Detection Err.} \\
       \textbf{OOD Method} &    \textbf{Layer}   &   Base &  Ctrst & $\Delta$ &      Base &  Ctrst & $\Delta$ &       Base &  Ctrst & $\Delta$ &           Base &  Ctrst & $\Delta$ &           Base &  Ctrst & $\Delta$ \\
\midrule
\textbf{Max Softmax} & \textbf{-} &  \underline{\textbf{96.04}} &  \underline{\textbf{96.15}} &     \textbf{0.11} &    \underline{\textbf{97.25}} &  \underline{\textbf{97.35}} &     \textbf{0.11} &      \underline{\textbf{93.46}} &  \underline{\textbf{93.45}} &    -0.02 &          \underline{\textbf{10.39}} &  \underline{\textbf{10.23}} &    \textbf{-0.16} &           \underline{\textbf{7.39}} &   \underline{\textbf{7.28}} &    \textbf{-0.11} \\
\textbf{Predictive Entropy} & \textbf{-} &  85.34 &  87.12 &     \textbf{1.78} &     89.42 &  91.06 &     \textbf{1.64} &      77.72 &  79.29 &     \textbf{1.58} &          35.55 &  30.10 &    \textbf{-5.45} &          20.15 &  17.22 &    \textbf{-2.92} \\
\textbf{Aleatoric Entropy} & \textbf{-} &  85.30 &  87.37 &     \textbf{2.06} &     89.07 &  90.98 &     \textbf{1.91} &      77.99 &  80.25 &     \textbf{2.26} &          37.87 &  30.76 &    \textbf{-7.11} &          21.34 &  17.69 &    \textbf{-3.65} \\
\textbf{Mutual Information} & \textbf{-} &  45.04 &  43.18 &    -1.86 &     44.13 &  43.54 &    -0.59 &      53.30 &  50.95 &    -2.35 &          98.75 &  98.66 &    \textbf{-0.09} &          49.99 &  49.99 &    -0.00 \\
\midrule
\multirow{6}{*}{\textbf{Mahalanobis}} & \textbf{logits} &  83.51 &  83.40 &    -0.11 &     81.04 &  80.53 &    -0.51 &      84.63 &  83.31 &    -1.32 &          66.26 &  69.77 &     3.51 &          35.55 &  37.31 &     1.75 \\
        & \textbf{backbone} &  \textbf{88.34} &  \textbf{89.88} &     \textbf{1.54} &     \textbf{89.99} &  \textbf{90.86} &     \textbf{0.87} &      \textbf{86.44} &  88.35 &     \textbf{1.90} &          \textbf{37.49} &  35.78 &    \textbf{-1.71} &          \textbf{21.16} &  20.29 &    \textbf{-0.87} \\
        & \textbf{conv2x} &  85.82 &  88.80 &     \textbf{2.98} &     84.44 &  85.90 &    \textbf{1.45} &      85.10 &  \textbf{89.61} &     \textbf{4.50} &          53.82 &  58.01 &     4.19 &          29.35 &  31.44 &     2.09 \\
        & \textbf{conv4x} &  72.57 &  80.11 &     \textbf{7.53} &     73.83 &  81.42 &     \textbf{7.60} &      68.86 &  77.10 &     \textbf{8.24} &          72.85 &  60.14 &   \textbf{-12.71} &          38.83 &  32.49 &    \textbf{-6.34} \\
        & \textbf{conv8x} &  67.08 &  71.82 &     \textbf{4.75} &     71.95 &  75.88 &     \textbf{3.93} &      58.73 &  63.58 &     \textbf{4.85} &          70.17 &  63.25 &    \textbf{-6.91} &          37.49 &  34.02 &    \textbf{-3.47} \\
        & \textbf{ctrst} &    - &  89.81 &      - &       - &  90.19 &      - &        - &  85.08 &      - &            - &  \textbf{35.07} &      - &            - &  \textbf{19.95} &      - \\
\midrule
\multirow{5}{*}{\textbf{OC-SVM}} & \textbf{logits} &  54.26 &  48.41 &    -5.85 &     51.69 &  47.02 &    -4.67 &      58.74 &  56.45 &    -2.29 &          96.38 &  97.57 &     1.19 &          49.53 &  49.84 &     0.31 \\
        & \textbf{conv2x} &  63.61 &  64.82 &     \textbf{1.21} &     77.11 &  76.76 &    -0.34 &      78.39 &  78.60 &     \textbf{0.22} &          68.39 &  \textbf{66.22} &    \textbf{-2.17} &          36.37 &  \textbf{35.43} &    \textbf{-0.94} \\
        & \textbf{conv4x} &  61.50 &  63.16 &     \textbf{1.66} &     74.71 &  76.27 &     \textbf{1.56} &      77.47 &  78.16 &     \textbf{0.69} &          77.32 &  71.20 &    \textbf{-6.12} &          40.91 &  37.92 &    \textbf{-2.99} \\
        & \textbf{conv8x} &  \textbf{66.49} &  63.12 &    -3.37 &     \textbf{82.29} &  \textbf{80.74} &    -1.55 &      \textbf{79.78} &  78.74 &    -1.04 &          \textbf{63.49} &  70.01 &     6.53 &          \textbf{33.61} &  36.92 &     3.30 \\
        & \textbf{ctrst} &    - &  \textbf{72.38} &      - &       - &  62.21 &      - &        - &  \textbf{79.69} &      - &            - &  93.43 &      - &            - &  48.82 &      - \\
\midrule
\multirow{6}{*}{\textbf{RealNVP}} & \textbf{logits} &  70.81 &  70.26 &    -0.55 &     74.09 &  73.57 &    -0.52 &      66.90 &  65.64 &    -1.26 &          68.84 &  69.44 &     0.60 &          36.82 &  37.10 &     0.28 \\
        & \textbf{backbone} &  93.63 &  92.50 &    -1.13 &     95.16 &  94.17 &    -0.99 &      90.82 &  89.22 &    -1.59 &          19.90 &  22.80 &     2.90 &          12.11 &  13.75 &     1.64 \\
        & \textbf{conv2x} &  92.07 &  93.59 &     \textbf{1.51} &     92.03 &  93.05 &     \textbf{1.03} &      91.43 &  92.66 &     \textbf{1.22} &          24.79 &  21.81 &    \textbf{-2.98} &          14.79 &  13.32 &   \textbf{-1.47} \\
        & \textbf{conv4x} &  \textbf{94.65} &  \textbf{95.79} &     \textbf{1.13} &     \textbf{95.92} &  \textbf{97.01} &     \textbf{1.09} &      \textbf{92.25} &  \textbf{92.78} &     \textbf{0.53} &          \textbf{17.85} &  \textbf{12.24} &    \textbf{-5.61} &          \textbf{11.12} &   \textbf{8.22} &    \textbf{-2.90} \\
        & \textbf{conv8x} &  88.96 &  84.02 &    -4.94 &     92.13 &  87.70 &    -4.42 &      80.85 &  76.57 &    -4.28 &          26.83 &  39.55 &    12.71 &          15.81 &  22.15 &     6.33 \\
        & \textbf{ctrst} &    - &  92.44 &      - &       - &  94.78 &      - &        - &  87.81 &      - &            - &  16.66 &      - &            - &  10.52 &      - \\
\bottomrule
\end{tabular}
\caption{Results for Carla objects}
\label{tab:full_results_carla}
\end{table*}

\begin{table*}
\centering
\tiny
\begin{tabular}{rc|ccc|ccc|ccc|ccc|ccc}
\toprule
        &       & \multicolumn{3}{c}{AUROC} & \multicolumn{3}{c}{AUPR (ID)} & \multicolumn{3}{c}{AUPR (OOD)} & \multicolumn{3}{c}{FPR @ 95\% TPR} & \multicolumn{3}{c}{Detection Err.} \\
       \textbf{OOD Method} &    \textbf{Layer}   &   Base &  Ctrst & $\Delta$ &      Base &  Ctrst & $\Delta$ &       Base &  Ctrst & $\Delta$ &           Base &  Ctrst & $\Delta$ &           Base &  Ctrst & $\Delta$ \\
\midrule
\textbf{Max Softmax} & \textbf{-} &  \underline{\textbf{95.38}} &  \underline{\textbf{96.06}} &     \textbf{0.48} &     \underline{\textbf{95.80}} &  \underline{\textbf{96.35}} &     \textbf{0.55} &      \underline{\textbf{95.32}} &  \underline{\textbf{95.77}} &     \textbf{0.45} &          \underline{\textbf{21.23}} &  \underline{\textbf{20.80}} &    \textbf{-0.43} &          \underline{\textbf{12.34}} &  \underline{\textbf{12.27}} &    \textbf{-0.08} \\
\textbf{Predictive Entropy} & \textbf{-} &  78.65 &  80.41 &     \textbf{1.76} &     84.83 &  86.59 &     \textbf{1.76} &      69.75 &  71.44 &     \textbf{1.69} &          41.66 &  36.10 &    \textbf{-5.55} &          22.74 &  20.01 &    \textbf{-2.73} \\
\textbf{Aleatoric Entropy} & \textbf{-} &  78.24 &  80.03 &     \textbf{1.79} &     84.31 &  86.11 &     \textbf{1.80} &      69.29 &  71.30 &     \textbf{2.01} &          43.93 &  38.59 &    \textbf{-5.33} &          24.00 &  21.26 &    \textbf{-2.73} \\
\textbf{Mutual Information} & \textbf{-} &  52.09 &  55.94 &     \textbf{3.86} &     47.53 &  50.16 &     \textbf{2.63} &      60.33 &  63.24 &     \textbf{2.91} &          99.13 &  98.58 &    \textbf{-0.55} &          49.95 &  49.96 &     0.01 \\
\midrule
\multirow{6}{*}{\textbf{Mahalanobis}} & \textbf{logits} &  74.12 &  78.08 &     \textbf{3.96} &     68.50 &  75.29 &     \textbf{6.79} &      73.93 &  75.74 &     \textbf{1.80} &          88.34 &  78.49 &    \textbf{-9.85} &          45.92 &  41.11 &    \textbf{-4.82} \\
        & \textbf{backbone} &  \textbf{86.25} &  84.09 &    -2.16 &     \textbf{86.07} &  85.46 &    -0.61 &      \textbf{85.98} &  83.46 &    -2.52 &          54.35 &  50.86 &    \textbf{-3.48} &          \textbf{28.80} &  27.18 &    \textbf{-1.62} \\
        & \textbf{conv2x} &  63.77 &  59.44 &    -4.33 &     62.04 &  59.80 &    -2.25 &      65.70 &  58.77 &    -6.93 &          90.77 &  88.91 &    \textbf{-1.86} &          46.81 &  46.23 &    \textbf{-0.58} \\
        & \textbf{conv4x} &  72.09 &  69.64 &    -2.44 &     70.67 &  67.15 &    -3.52 &      72.15 &  67.54 &    -4.62 &          78.82 &  84.29 &     5.47 &          41.25 &  43.94 &     2.68 \\
        & \textbf{conv8x} &  85.02 &  89.98 &     \textbf{4.96} &     84.94 &  \textbf{91.84} &     \textbf{6.90} &      80.52 &  85.98 &     \textbf{5.47} &          \textbf{55.34} &  32.50 &   \textbf{-22.84} &          29.25 &  18.32 &   \textbf{-10.93} \\
        & \textbf{ctrst} &    - &  \textbf{93.76} &      - &       - &  91.28 &      - &        - &  \textbf{93.09} &      - &            - &  \textbf{29.12} &      - &            - &  \textbf{16.06} &      - \\
\midrule
\multirow{5}{*}{\textbf{OCSVM}} & \textbf{logits} &  51.71 &  59.31 &     \textbf{7.60} &     51.22 &  61.06 &     \textbf{9.84} &      51.36 &  57.29 &     \textbf{5.93} &          95.39 &  78.44 &   \textbf{-16.95} &          49.11 &  41.15 &    \textbf{-7.97} \\
        & \textbf{conv2x} &  57.65 &  57.45 &    -0.20 &     61.82 &  61.07 &    -0.74 &      73.69 &  72.69 &    -1.01 &          90.26 &  88.26 &    \textbf{-2.00} &          46.62 &  46.17 &    \textbf{-0.46} \\
        & \textbf{conv4x} &  63.44 &  64.52 &     \textbf{1.08} &     80.73 &  80.64 &    -0.09 &      78.76 &  79.12 &     \textbf{0.37} &          69.34 &  67.22 &    \textbf{-2.11} &          36.61 &  35.52 &    \textbf{-1.08} \\
        & \textbf{conv8x} &  \textbf{66.95} &  63.67 &    -3.28 &     \textbf{82.44} &  81.83 &    -0.60 &      \textbf{80.00} &  79.03 &    -0.98 &          \textbf{62.58} &  69.03 &     6.45 &          \textbf{33.10} &  36.33 &     3.23 \\
        & \textbf{ctrst} &    - &  \textbf{93.13} &      - &       - &  \textbf{92.67} &      - &        - &  \textbf{94.06} &      - &            - &  \textbf{25.98} &      - &            - &  \textbf{15.02} &      - \\
\midrule
\multirow{6}{*}{\textbf{RealNVP}} & \textbf{logits} &  80.52 &  76.22 &    -4.29 &     79.61 &  77.48 &    -2.12 &      79.82 &  73.18 &    -6.64 &          67.14 &  67.79 &     0.64 &          35.56 &  35.83 &     0.28 \\
        & \textbf{backbone} &  85.81 &  84.02 &    -1.79 &     90.13 &  89.09 &    -1.04 &      77.69 &  74.08 &    -3.61 &          31.17 &  32.49 &     1.31 &          17.49 &  18.18 &     0.69 \\
        & \textbf{conv2x} &  77.66 &  76.60 &    -1.06 &     75.72 &  76.39 &     \textbf{0.67} &      76.83 &  73.24 &    -3.59 &          70.63 &  71.81 &     1.18 &          37.33 &  37.73 &     0.40 \\
        & \textbf{conv4x} &  \textbf{92.30} &  91.79 &    -0.52 &     \textbf{92.84} &  92.93 &     \textbf{0.09} &      \textbf{90.32} &  88.48 &    -1.84 &          \textbf{27.39} &  34.80 &     7.42 &          \textbf{15.63} &  19.24 &     3.61 \\
        & \textbf{conv8x} &  90.10 &  87.13 &    -2.98 &     91.97 &  91.08 &    -0.89 &      85.62 &  80.26 &    -5.37 &          34.80 &  28.58 &    \textbf{-6.22} &          19.29 &  16.23 &    \textbf{-3.06} \\
        & \textbf{ctrst} &    - &  \textbf{94.79} &      - &       - &  \textbf{95.23} &      - &        - &  \textbf{92.62} &      - &            - &  \textbf{23.55} &      - &            - &  \textbf{13.62} &      - \\
\bottomrule
\end{tabular}
\caption{Results for KITTI ignored objects}
\label{tab:full_results_ignored}
\end{table*}

\begin{table*}
\centering
\tiny
\begin{tabular}{rc|ccc|ccc|ccc|ccc|ccc}
\toprule
        &       & \multicolumn{3}{c}{AUROC} & \multicolumn{3}{c}{AUPR (ID)} & \multicolumn{3}{c}{AUPR (OOD)} & \multicolumn{3}{c}{FPR @ 95\% TPR} & \multicolumn{3}{c}{Detection Err.} \\
       \textbf{OOD Method} &    \textbf{Layer}   &   Base &  Ctrst & $\Delta$ &      Base &  Ctrst & $\Delta$ &       Base &  Ctrst & $\Delta$ &           Base &  Ctrst & $\Delta$ &           Base &  Ctrst & $\Delta$ \\
\midrule
\textbf{Max Softmax} & \textbf{-} &  82.84 &  82.87 &     \textbf{0.03} &     88.06 &  88.36 &     \textbf{0.30} &      72.43 &  72.06 &    -0.37 &          36.41 &  34.05 &    \textbf{-2.36} &          20.64 &  19.40 &    \textbf{-1.23} \\
\textbf{Predictive Entropy} & \textbf{-} &  86.92 &  86.76 &    -0.16 &     90.83 &  90.93 &     \textbf{0.11} &      80.34 &  79.32 &    -1.02 &          29.69 &  27.96 &    \textbf{-1.73} &          17.22 &  16.23 &    \textbf{-0.99} \\
\textbf{Aleatoric Entropy} & \textbf{-} &  86.76 &  86.77 &     \textbf{0.02} &     90.69 &  90.90 &     \textbf{0.20} &      79.87 &  79.48 &    -0.39 &          30.09 &  28.24 &    \textbf{-1.86} &          17.44 &  16.37 &    \textbf{-1.07} \\
\textbf{Mutual Information} & \textbf{-} &  70.62 &  72.47 &     \textbf{1.86} &     66.79 &  69.55 &     \textbf{2.76} &      68.34 &  69.49 &     \textbf{1.15} &          85.78 &  82.66 &    \textbf{-3.12} &          45.37 &  43.82 &    \textbf{-1.55} \\
\midrule
\multirow{6}{*}{\textbf{Mahalanobis}} & \textbf{logits} &  47.34 &  49.66 &     \textbf{2.32} &     46.27 &  46.62 &     \textbf{0.34} &      52.99 &  55.72 &     \textbf{2.73} &          97.17 &  97.66 &     0.49 &          49.97 &  49.98 &     0.01 \\
        & \textbf{backbone} &  72.48 &  \textbf{80.60} &     \textbf{8.11} &     78.11 &  \textbf{86.52} &     \textbf{8.41} &      64.03 &  70.88 &     \textbf{6.85} &          59.52 &  \textbf{38.05} &   \textbf{-21.47} &          32.24 &  \textbf{21.43} &   \textbf{-10.80} \\
        & \textbf{conv2x} &  \textbf{76.18} &  79.94 &     \textbf{3.76} &     \textbf{81.64} &  85.00 &     \textbf{3.36} &      \textbf{67.34} & \textbf{ 72.18} &     \textbf{4.84} &          \textbf{53.12} &  44.72 &    \textbf{-8.40} &          \textbf{29.04} &  24.81 &    \textbf{-4.22} \\
        & \textbf{conv4x} &  47.69 &  55.70 &     \textbf{8.01} &     48.95 &  57.91 &     \textbf{8.96} &      47.58 &  51.88 &     \textbf{4.30} &          95.06 &  87.64 &    \textbf{-7.42} &          49.65 &  46.26 &    \textbf{-3.38} \\
        & \textbf{conv8x} &  42.91 &  51.91 &     \textbf{9.01} &     45.67 &  55.59 &     \textbf{9.92} &      44.45 &  49.29 &     \textbf{4.85} &          96.30 &  89.28 &    \textbf{-7.02} &          49.66 &  47.03 &    \textbf{-2.63} \\
        & \textbf{ctrst} &    &  50.02 &      - &       - &  52.86 &      - &        - &  49.30 &      - &            - &  90.70 &      - &            - &  46.57 &      - \\
\midrule
\multirow{5}{*}{\textbf{OC-SVM}} & \textbf{logits} &  54.72 &  35.60 &   -19.13 &     61.71 &  52.18 &    -9.53 &      63.23 &  50.06 &   -13.16 &          \textbf{67.89} &  \textbf{70.61} &     2.71 &          \textbf{34.76} &  \textbf{35.81} &     1.06 \\
        & \textbf{conv2x} &  54.35 &  57.45 &     \textbf{3.10} &     61.80 &  65.80 &     \textbf{4.00} &      70.37 &  72.34 &    \textbf{ 1.97} &          82.22 &  78.88 &    \textbf{-3.34} &          43.36 &  41.56 &    \textbf{-1.80} \\
        & \textbf{conv4x} &  23.16 &  24.00 &     \textbf{0.84} &     33.50 &  33.82 &     \textbf{0.33} &      46.59 &  47.40 &     \textbf{0.81} &          99.29 &  99.26 &    \textbf{-0.03} &          50.00 &  49.99 &    -0.00 \\
        & \textbf{conv8x} &  \textbf{63.22} &  \textbf{62.59} &    -0.63 &     \textbf{73.98} &  \textbf{79.64} &     \textbf{5.66} &      \textbf{77.07} &  \textbf{78.42} &     \textbf{1.35} &          72.03 &  70.91 &    \textbf{-1.11} &          38.34 &  37.48 &    \textbf{-0.87} \\
        & \textbf{ctrst} &    - &  10.30 &      - &       - &  32.18 &      - &        - &  32.49 &      - &            - &  99.40 &      - &            - &  50.00 &      - \\
\midrule
\multirow{6}{*}{\textbf{RealNVP}} & \textbf{logits} &  45.35 &  43.23 &    -2.11 &     48.57 &  48.00 &    -0.57 &      46.32 &  44.59 &    -1.73 &          94.23 &  94.18 &    \textbf{-0.05} &          48.17 &  48.88 &     0.71 \\
        & \textbf{backbone} &  \underline{\textbf{91.71}} &  \underline{\textbf{91.81}} &     \textbf{0.10} &     \underline{\textbf{94.69}} &  \underline{\textbf{94.79}} &     \textbf{0.09} &      \underline{\textbf{84.77}} &  \underline{\textbf{85.44}} &    \textbf{0.67} &          \underline{\textbf{16.25}} &  \underline{\textbf{15.44}} &    \textbf{-0.81} &           \underline{\textbf{9.58}} &   \underline{\textbf{8.99}} &    \textbf{-0.59} \\
        & \textbf{conv2x} &  60.67 &  77.25 &    \textbf{16.58} &     68.26 &  83.51 &    \textbf{15.25} &      57.28 &  68.29 &    \textbf{11.01} &          65.80 &  46.29 &   \textbf{-19.51} &          34.96 &  25.48 &    \textbf{-9.48} \\
        & \textbf{conv4x} &  70.46 &  74.13 &     \textbf{3.66} &     77.83 &  80.92 &     \textbf{3.09} &      62.13 &  65.78 &     \textbf{3.65} &          57.30 &  48.94 &    \textbf{-8.36} &          31.00 &  26.36 &    \textbf{-4.64} \\
        & \textbf{conv8x} &  77.71 &  78.96 &    \textbf{1.25} &     84.86 &  83.63 &    -1.23 &      66.30 &  71.48 &     \textbf{5.18} &          40.53 &  40.06 &    \textbf{-0.47} &          22.53 &  21.62 &    \textbf{-0.92} \\
        & \textbf{ctrst} &    - &  80.91 &      - &       - &  88.48 &      - &        - &  66.52 &      - &            - &  27.81 &      - &            - &  14.51 &      - \\
\bottomrule
\end{tabular}
\caption{Results for KITTI FP objects}
\label{tab:full_results_fp}
\end{table*}

\begin{table*}
\centering
\tiny
\begin{tabular}{rc|ccc|ccc|ccc|ccc|ccc}
\toprule
        &       & \multicolumn{3}{c}{AUROC} & \multicolumn{3}{c}{AUPR (ID)} & \multicolumn{3}{c}{AUPR (OOD)} & \multicolumn{3}{c}{FPR @ 95\% TPR} & \multicolumn{3}{c}{Detection Err.} \\
       \textbf{OOD Method} &    \textbf{Layer}   &   Base &  Ctrst & $\Delta$ &      Base &  Ctrst & $\Delta$ &       Base &  Ctrst & $\Delta$ &           Base &  Ctrst & $\Delta$ &           Base &  Ctrst & $\Delta$ \\
\midrule
\textbf{Max Softmax} & \textbf{-} &  83.18 &  83.34 &     \textbf{0.16} &     85.41 &  86.51 &    \textbf{1.10} &      78.72 &  78.23 &    -0.49 &          52.17 &  45.80 &    \textbf{-6.36} &          28.53 &  25.35 &    \textbf{-3.18} \\
\textbf{Predictive Entropy} & \textbf{-} &  80.64 &  81.23 &     \textbf{0.58} &     83.86 &  85.29 &     \textbf{1.43} &      74.48 &  74.49 &     \textbf{0.01} &          53.69 &  47.50 &    \textbf{-6.19} &          29.29 &  26.19 &    \textbf{-3.10} \\
\textbf{Aleatoric Entropy} & \textbf{-} &  80.01 &  80.90 &     \textbf{0.88} &     83.45 &  85.05 &     \textbf{1.61} &      73.14 &  73.96 &     \textbf{0.82} &          53.97 &  47.62 &    \textbf{-6.36} &          29.44 &  26.27 &    \textbf{-3.17} \\
\textbf{Mutual Information} & \textbf{-} &  67.53 &  66.41 &    -1.12 &     63.31 &  63.70 &     \textbf{0.39} &      67.16 &  65.15 &    -2.01 &          90.14 &  86.23 &    \textbf{-3.91} &          47.50 &  45.56 &    \textbf{-1.93} \\
\midrule
\multirow{6}{*}{\textbf{Mahalanobis}} & \textbf{logits} &  52.45 &  52.37 &    -0.09 &     49.40 &  47.05 &    -2.36 &      58.55 &  62.28 &     \underline{\textbf{3.73}} &          96.29 &  98.21 &     1.93 &          49.73 &  49.98 &     0.25 \\
        & \textbf{backbone} &  \textbf{88.30} &  \textbf{82.21} &    -6.09 &     \textbf{88.59} &  \textbf{83.27} &    -5.32 &      \textbf{85.96} &  79.16 &    -6.80 &          \textbf{43.53} &  \textbf{51.34} &     7.80 &          \textbf{24.22} &  \textbf{28.11} &     3.89 \\
        & \textbf{conv2x} &  85.96 &  81.80 &    -4.16 &     85.04 &  80.29 &    -4.75 &      83.49 &  \textbf{79.77} &    -3.72 &          54.93 &  66.69 &    11.76 &          29.94 &  35.81 &     5.88 \\
        & \textbf{conv4x} &  73.61 &  69.04 &    -4.57 &     70.75 &  64.27 &    -6.48 &      72.48 &  69.60 &    -2.88 &          81.35 &  89.39 &     8.04 &          43.10 &  47.11 &     4.00 \\
        & \textbf{conv8x} &  69.90 &  71.70 &     \textbf{1.80} &     71.88 &  73.19 &     \textbf{1.31} &      63.76 &  65.78 &     \textbf{2.01} &          75.88 &  73.17 &    \textbf{-2.71} &          40.39 &  39.04 &    \textbf{-1.36} \\
        & \textbf{ctrst} &    - &  70.37 &      - &       - &  64.18 &      - &        - &  69.45 &      - &            - &  92.54 &      - &            - &  48.44 &      - \\
\midrule
\multirow{5}{*}{\textbf{OCSVM}} & \textbf{logits} &  48.13 &  55.08 &     \textbf{6.96} &     50.58 &  53.44 &     \textbf{2.86} &      47.96 &  56.23 &     \textbf{8.28} &          90.63 &  91.87 &     1.24 &          46.93 &  47.87 &     0.93 \\
        & \textbf{conv2x} &  63.66 &  64.51 &     \textbf{0.85} &     77.92 &  76.58 &    -1.34 &      \textbf{78.49} &  \textbf{78.42} &    -0.07 &          68.43 &  \textbf{66.47} &    \textbf{-1.96} &          36.33 &  \textbf{35.62} &    \textbf{-0.72} \\
        & \textbf{conv4x} &  62.36 &  62.95 &    \textbf{0.59} &     \textbf{78.15} &  76.19 &    -1.96 &      78.21 &  78.08 &    -0.13 &          71.18 &  69.82 &    \textbf{-1.36} &          37.65 &  37.27 &    \textbf{-0.39} \\
        & \textbf{conv8x} &  \textbf{64.74} &  62.20 &    -2.55 &     78.02 &  \textbf{78.00} &    -0.02 &      78.35 &  78.07 &    -0.28 &          \textbf{67.81} &  71.51 &     3.70 &          \textbf{36.17} &  37.94 &     1.77 \\
        & \textbf{ctrst} &    - &  \textbf{76.53} &      - &       - &  72.76 &      - &        - &  77.67 &      - &            - &  87.44 &      - &            - &  45.66 &      - \\
\midrule
\multirow{6}{*}{\textbf{RealNVP}} & \textbf{logits} &  59.93 &  55.35 &    -4.59 &     62.04 &  53.92 &    -8.12 &      57.74 &  54.51 &    -3.23 &          84.17 &  93.10 &     8.93 &          44.51 &  48.59 &     4.08 \\
        & \textbf{backbone} &  85.44 &  79.56 &    -5.88 &     89.46 &  84.60 &    -4.86 &      80.73 &  74.04 &    -6.69 &          33.03 &  46.01 &    12.98 &          18.92 &  25.43 &     6.51 \\
        & \textbf{conv2x} &  84.62 &  82.29 &    -2.33 &     85.65 &  83.18 &    -2.47 &      82.17 &  79.84 &    -2.34 &          51.38 &  57.98 &     6.61 &          28.14 &  31.46 &     3.32 \\
        & \textbf{conv4x} &  \underline{\textbf{91.45}} &  \underline{\textbf{88.93}} &    -2.53 &    \underline{\textbf{92.77}} &  \underline{\textbf{89.76}} &    -3.01 &      \underline{\textbf{88.86}} &  \underline{\textbf{86.86}} &    -2.00 &  \underline{\textbf{31.47}} &  \underline{\textbf{44.45}} &    12.98 &  \underline{\textbf{18.18}} &  \underline{\textbf{24.68}} &     6.50 \\
        & \textbf{conv8x} &  78.69 &  74.58 &    -4.10 &     82.43 &  79.87 &    -2.55 &      71.27 &  66.54 &    -4.74 &          54.13 &  56.44 &     2.30 &          29.52 &  30.67 &     1.15 \\
        & \textbf{ctrst} &    - &  79.28 &      - &       - &  79.32 &      - &        - &  74.74 &      - &            - &  65.70 &      - &            - &  35.31 &      - \\
\bottomrule
\end{tabular}
\caption{Results for Waymo objects}
\label{tab:full_results_waymo}
\end{table*}

\subsection{Complete results}
\Cref{tab:full_results_all} shows the additional results with all evaluation
metrics and additional layers for all common OOD objects (i.e., OOD objects that
are detected by both the base model and the contrastive model for a given run)
for all OOD datasets. Results separated for each OOD dataset are in
\cref{tab:full_results_carla,tab:full_results_ignored,tab:full_results_fp,tab:full_results_waymo}.
We highlight two additional observations.

For Mahalanobis distance and normalizing flows, backbone layer provides best
overall performance. However, the optimal layer can vary for different type of
OOD objects. For instance, for KITTI ignored and Waymo objects
(\Cref{tab:full_results_ignored,tab:full_results_waymo}), using normalizing
flows with conv4x features gives better results than with backbone features,
whereas for KITTI FP objects (\Cref{tab:full_results_fp}), backbone layer has
20\% higher AUROC and AUPR compared to conv4x layer. For Mahalanobis distance,
the variation is smaller. Conv2x layer provides better performance for a few
metrics than backbone layer for Carla and KITTI FP objects
(\cref{tab:full_results_carla,tab:full_results_fp}).

For the contrastive model, we also utilize the contrastive layer features
(labeled `ctrst' in the table) to train Mahalanobis distance, OC-SVM, and
normalizing flows. The contrastive layer does not provide a consistent overall
improvement for any of the methods over all types of OOD objects
(\Cref{tab:full_results_all}). Interestingly, for KITTI ignored objects
(\Cref{tab:full_results_ignored}), the contrastive layer is the best performing
layer for all three methods, outperforming other layers by a large margin. This
suggests that the contrastive features are highly biased towards certain types
of OOD objects. It would be interesting to investigate whether or not this issue
also exists for image-based object detection and classification.

\subsection{Performance impact of OOD detection}
To demonstrate how OOD detection would impact the object detector's performance
during deployment, we evaluate the mAP performance of the base model on KITTI
moderate objects after removing predictions with OOD scores higher than a
threshold. This is done across multiple OOD score thresholds. We choose
normalizing flows (RealNVP) with the backbone layer as our OOD detector, which
has the best overall performance for the base model. We use one set of
experiments with the dataset augmented with Carla, KITTI FP, KITTI Ignored, and
Waymo objects. \Cref{fig:performance_impact} shows the mAP, number of FP, and
number of OOD across multiple OOD score thresholds.

With a lower OOD score threshold, more predictions are marked as OOD objects,
which naturally eliminates more FP and OOD objects but introduces more FN at the
same time, leading to a decrease in mAP performance. From
\Cref{fig:performance_impact}, we see that with 2\% mAP performance decrease,
over 50\% of the FP can be eliminated. However, the OOD recall varies
significantly for different types of OOD objects. Overall, 35.3\% of the objects
labeled as OOD can be successfully identified, which shows that the OOD
detection method is a practical addition to a 3D object detector in deployment.

\begin{figure}
    \centering
    \begin{subfigure}[b]{0.49\linewidth}
        \centering
        \includegraphics[width=\textwidth]{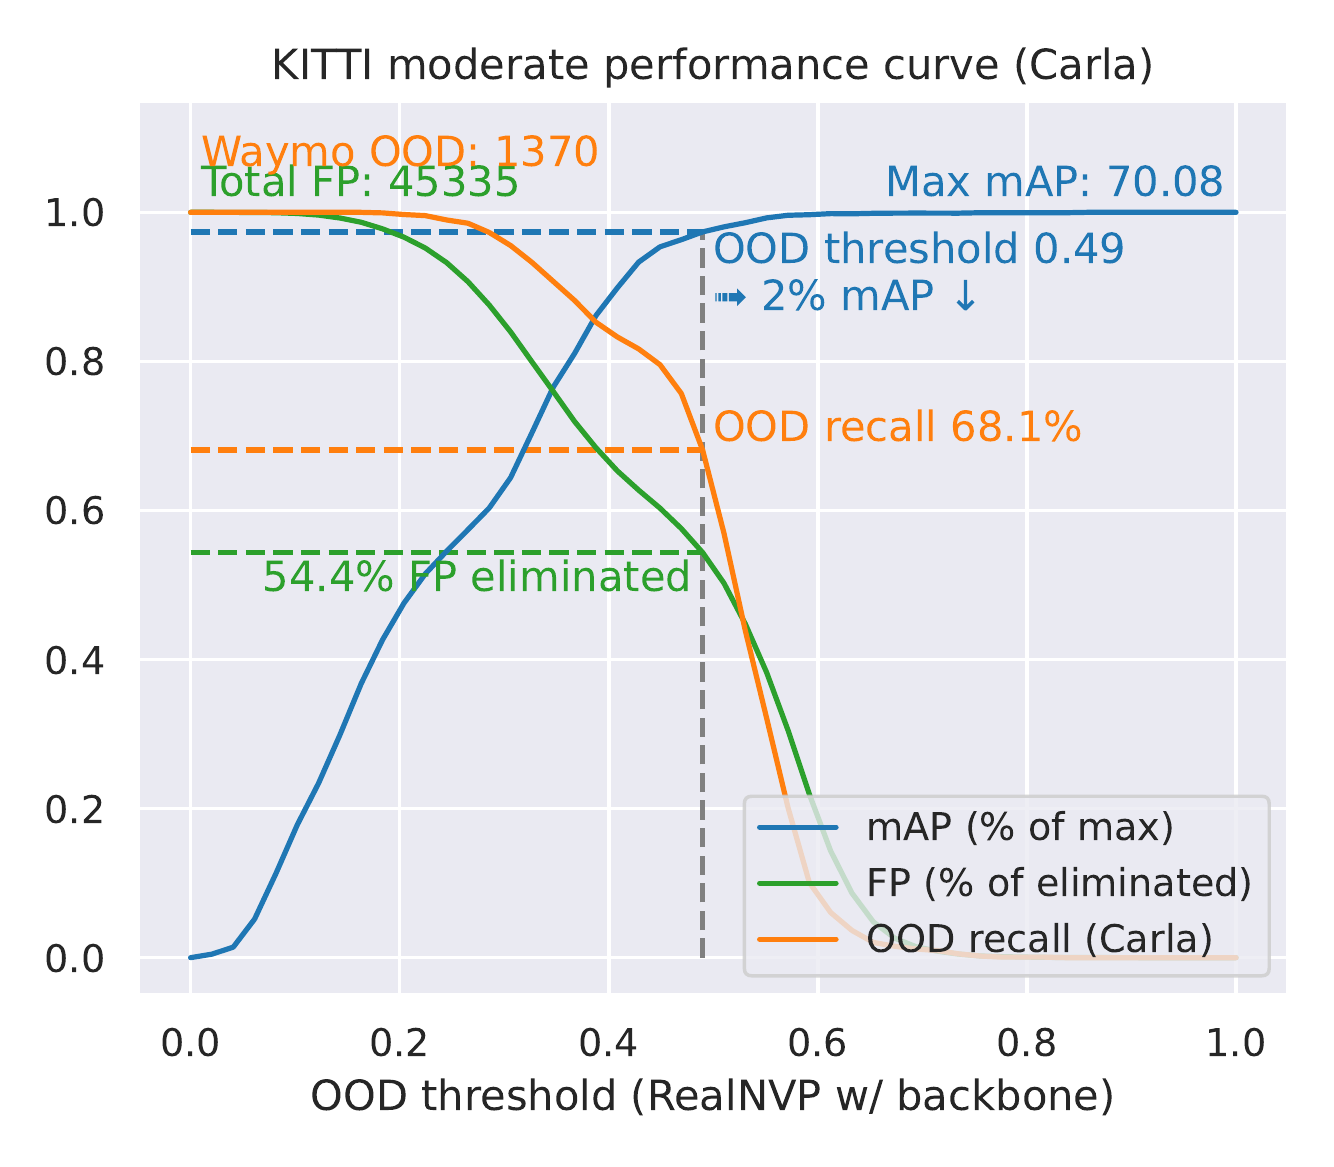}
        \caption{Carla}
    \end{subfigure}
    \begin{subfigure}[b]{0.49\linewidth}
        \centering
        \includegraphics[width=\textwidth]{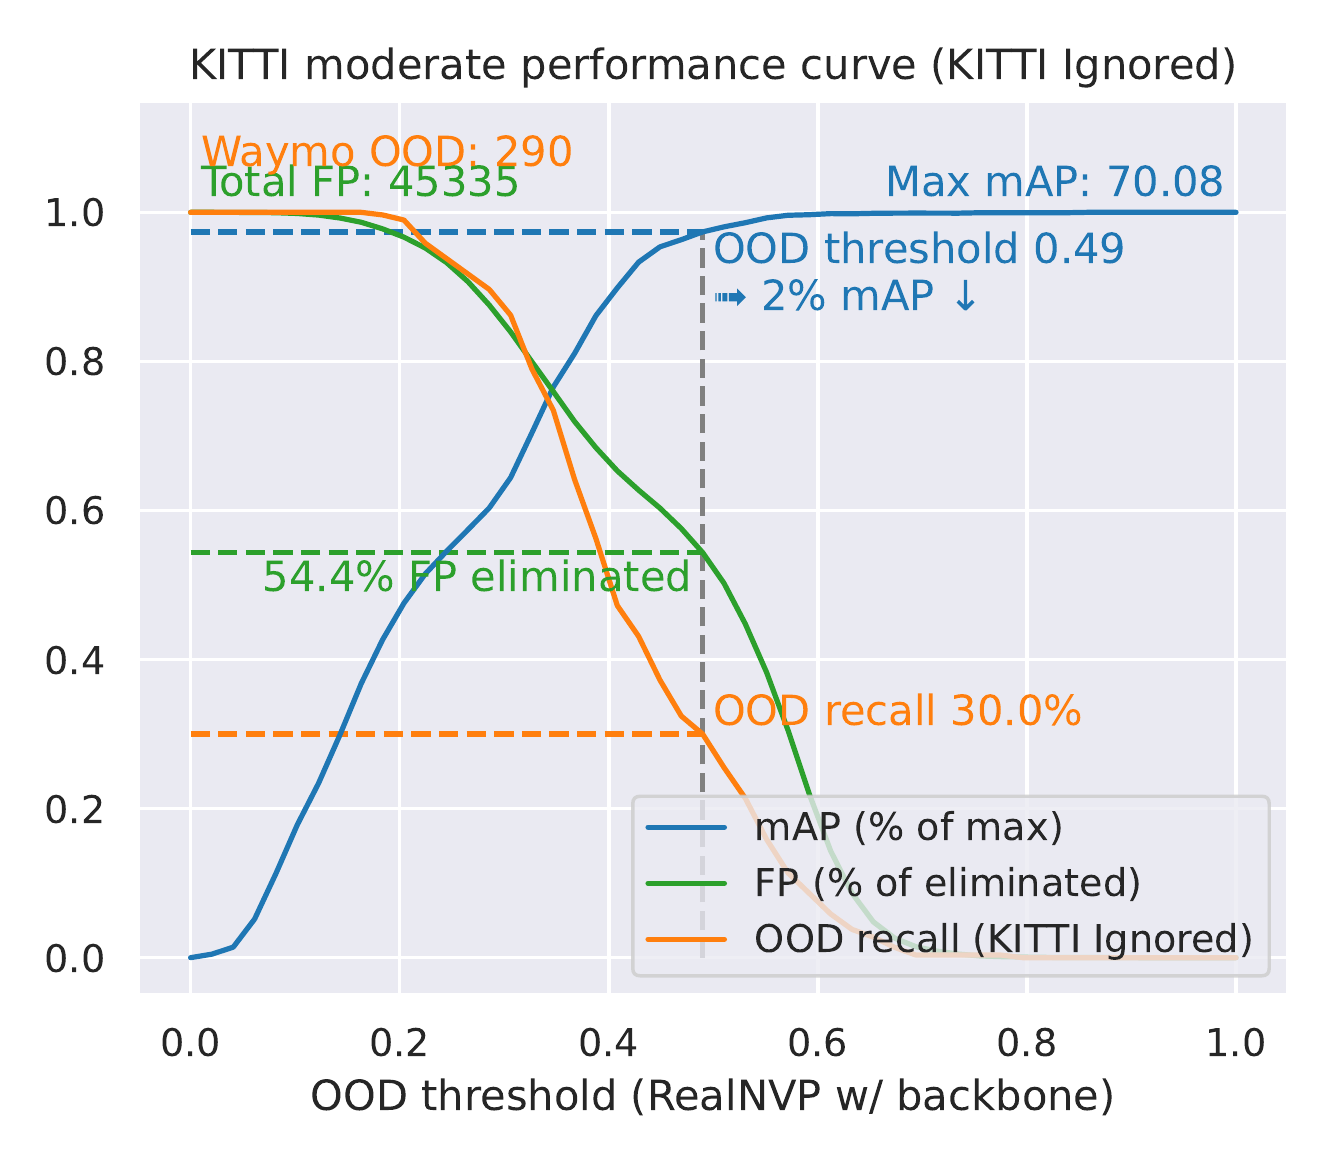}
        \caption{KITTI Ignored}
    \end{subfigure}
    \begin{subfigure}[b]{0.49\linewidth}
        \centering
        \includegraphics[width=\textwidth]{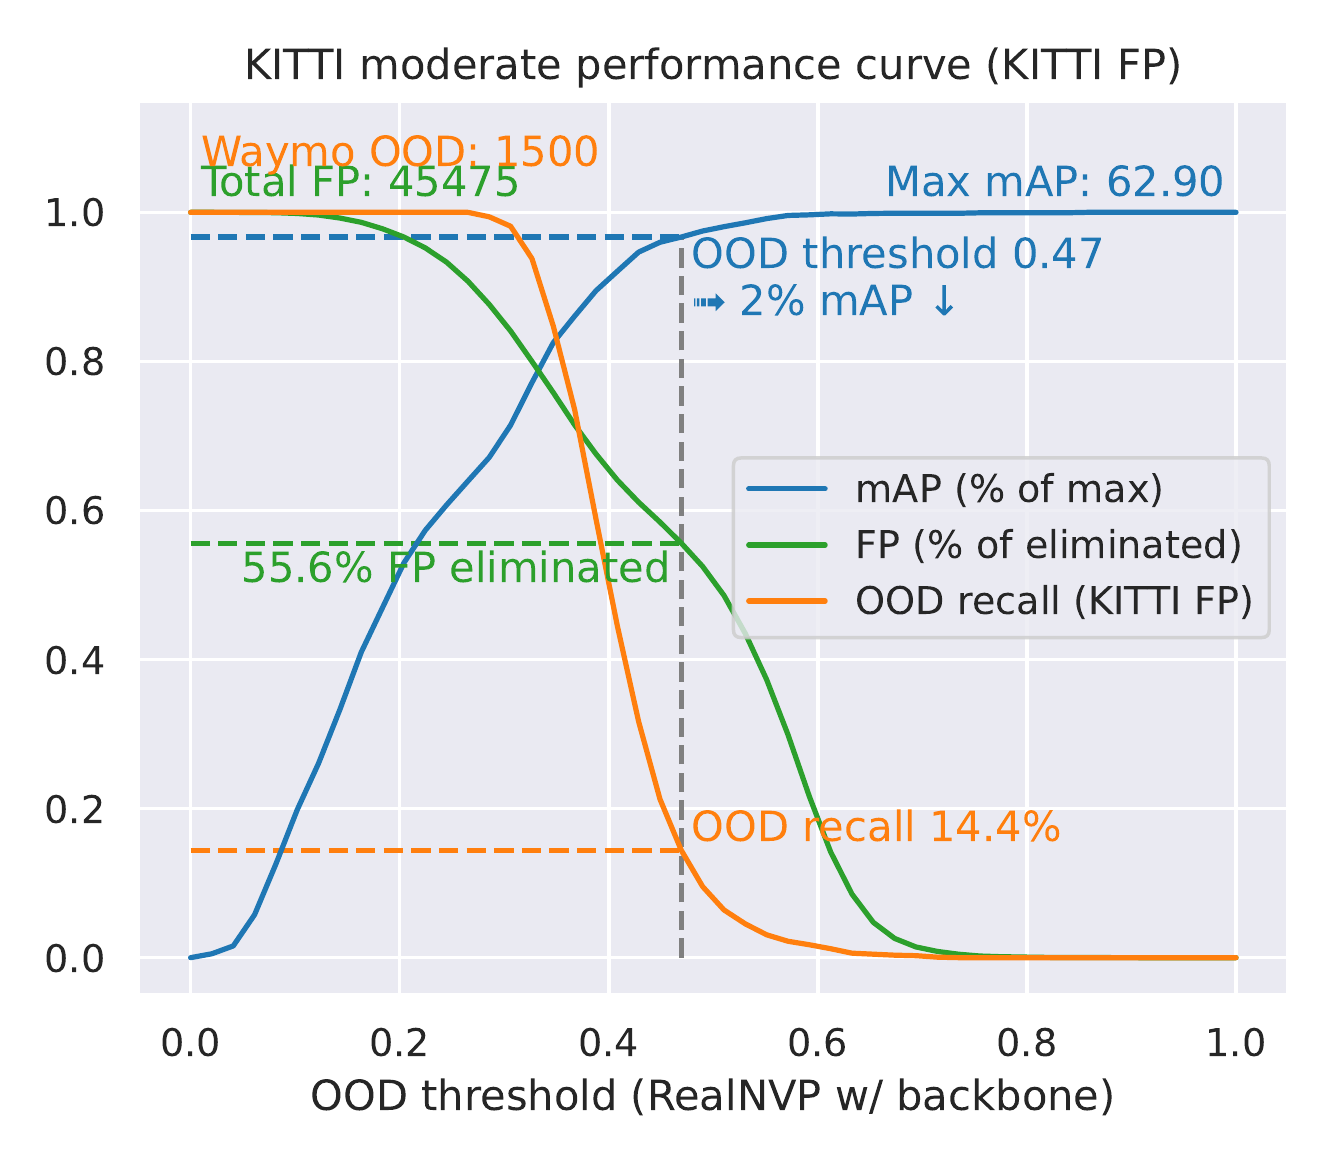}
        \caption{KITTI FP}
    \end{subfigure}
    \begin{subfigure}[b]{0.49\linewidth}
        \centering
        \includegraphics[width=\textwidth]{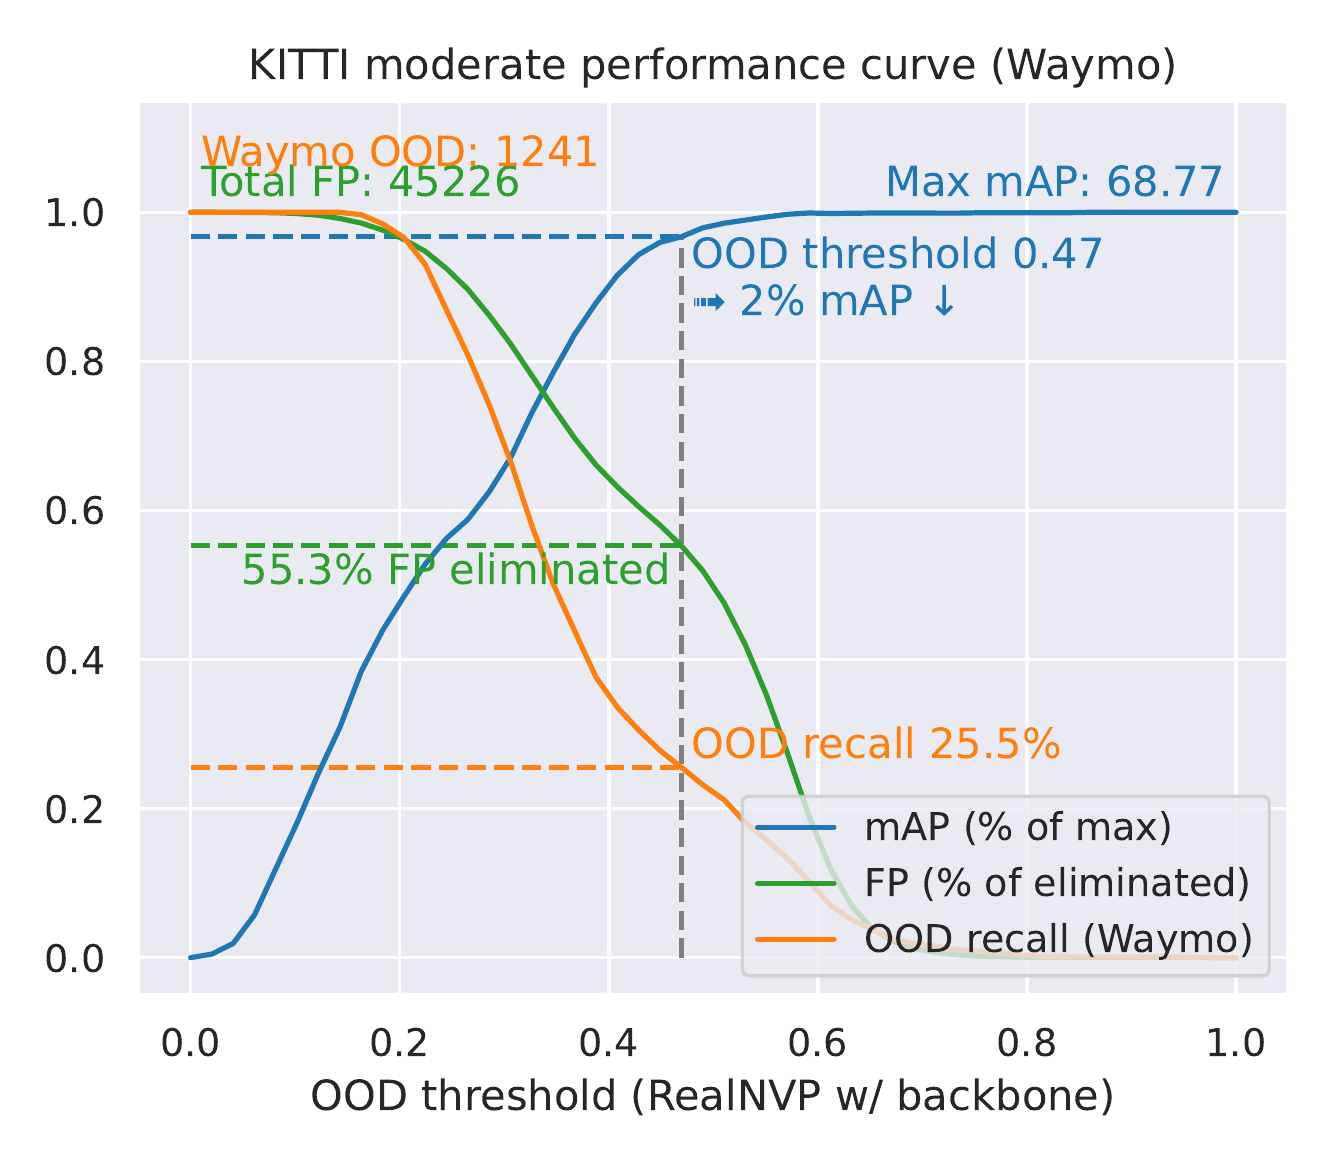}
        \caption{Waymo}
    \end{subfigure}
    \caption{Performance impact of OOD detection.}
    \label{fig:performance_impact}
\end{figure}

\subsection{Qualitative results}
\Cref{fig:qualitative} shows the qualitative results for OOD detection with
max-softmax score and normalizing flows OOD detection methods. We use the base
model without contrastive learning and normalizing flows with the backbone
layer, which has the best overall performance for the base model
(\Cref{tab:full_results_all}). For each type of OOD objects, we show three
examples: successful detection, normalizing flows (RealNVP) failure, and
max-softmax failure. Successful detections are examples where the OOD object is
assigned low max-softmax score and high OOD score; RealNVP failures are examples
where the OOD score from the normalizing flows for the OOD object is lower than
ID objects; Max-softmax failures are examples where the max-softmax score for
OOD object is higher than ID objects.

\begin{figure*}
    \centering
    \includegraphics[width=0.8\textwidth]{fig/qualitative.pdf}
    \caption{Qualitative results for OOD detection with max-softmax and OOD scores from normalizing flows (RealNVP) with backbone layer. Red boxes represents ground truth ID objects, yellow boxes are OOD objects, and green boxes are predictions from the base model. The text labels for RealNVP and max-softmax failures are red.}
    \label{fig:qualitative}
\end{figure*}

\section{Dataset description}
We present \Cref{alg:cap} to generate an OOD dataset for a model from an OOD
object database and an ID dataset. It takes an ID dataset, an OOD object
database, an object detection model, and two parameters: maximum number of
trials $\gamma_{max}$ and maximum number of objects $\zeta_{max}$ as inputs. The
output is an OOD dataset that includes ID objects from the ID dataset and OOD
objects from the OOD object database. We also provide a diagram in
\Cref{fig:ood_gen_diagram} describing the OOD dataset generation process.
% \begin{algorithm}[t] \scriptsize \caption{OOD dataset
% generation}\label{alg:cap_harry} \begin{algorithmic}[1] \Require ID dataset,
% OOD object database, an object detection model,  $\gamma_{max}$, $\zeta_{max}$
% \Ensure OOD dataset \Function {OODDatasetGeneration}{} \For {each class $\in$
% OOD database} \State $\zeta \leftarrow 0$ \For {a random frame $\in$ ID
% dataset and $\zeta \leq \zeta_{max}$} \State perform inference to get existing
% predictions \State $\gamma  \leftarrow 0 $ \While {$\gamma \leq \gamma_{max}$}
% \State select randomly an object $\in$ class \State select randomly an
% relative angle \State add object to frame \If{\textit{IoU}(object, existing
% ground truths and predictions) $\neq 0$, \State or object $\notin$ the FOV
% range} \State $\gamma \leftarrow \gamma + 1$ \State \textbf{continue} \EndIf
% \If {object not detected by model} \State $\gamma \leftarrow \gamma + 1$
% \State \textbf{continue} \Else \State object successfully added \State $\gamma
% \leftarrow \gamma + 1$ \State $\zeta \leftarrow \zeta + 1$ \State
% \textbf{break} \EndIf \EndWhile \EndFor \EndFor \EndFunction \end{algorithmic}
% \end{algorithm}
\begin{algorithm}[H]
\scriptsize
\caption{OOD dataset generation}\label{alg:cap}
\begin{algorithmic}[1]
    \Require ID dataset ($I$), OOD object database ($O$), detection model ($M$),
    maximum number of attempt $\gamma_{max}$, maximum number of OOD objects
    ($\zeta_{max}$) \Ensure OOD dataset ($I$) \Function {OODGenerator
    }{$I$,$O$,$M$,$\gamma_{max}$, $\zeta_{max}$ } \For {$c \in classes(O$)}
    \State $\zeta \gets 0$ \For {$f \in I$ \textbf{and} $\zeta \leq
    \zeta_{max}$} \State $P \gets M(f)$ \Comment{obtain predictions} \State
    $\gamma  \gets 0 $ \While {$\gamma \leq \gamma_{max}$} \State $o \gets
    rand\_obj(c)$ \Comment{select an object $\in c$} \State $a \gets
    rand\_angle()$\Comment{select an relative angle} \State $f^{\prime} \gets
    insert(f,o,a)$ \Comment{add object to frame}

            \If{\textit{IoU}($o$, GT($f$), $P$) $\neq 0$ \textbf{or} $o$
                \textbf{is not in} the FOV range} \\ \Comment{GT returns ground
                truth objects} \State $\gamma \gets \gamma + 1$ \State
                \textbf{continue} \EndIf \State $P^{\prime} \gets
                \textit{M}(f^{\prime})$ \Comment{obtain predictions} \If {$o
                \notin P^{\prime}$ } \State $\gamma \gets \gamma + 1$ \State
                \textbf{continue} \Else \State $I \gets update(f^{\prime},I)$
                \Comment{update the dataset} \State $\gamma \gets \gamma + 1$
                \State $\zeta \gets \zeta + 1$ \State \textbf{break} \EndIf
                \EndWhile \EndFor \EndFor \State \textbf{return} $I$
                \EndFunction

\end{algorithmic}
\end{algorithm}
\begin{figure*}[t]
\begin{center}
% \begin{overpic} 
% [width=\linewidth]
% {example-image-a}
% \end{overpic}
\includegraphics[width=0.8\textwidth]{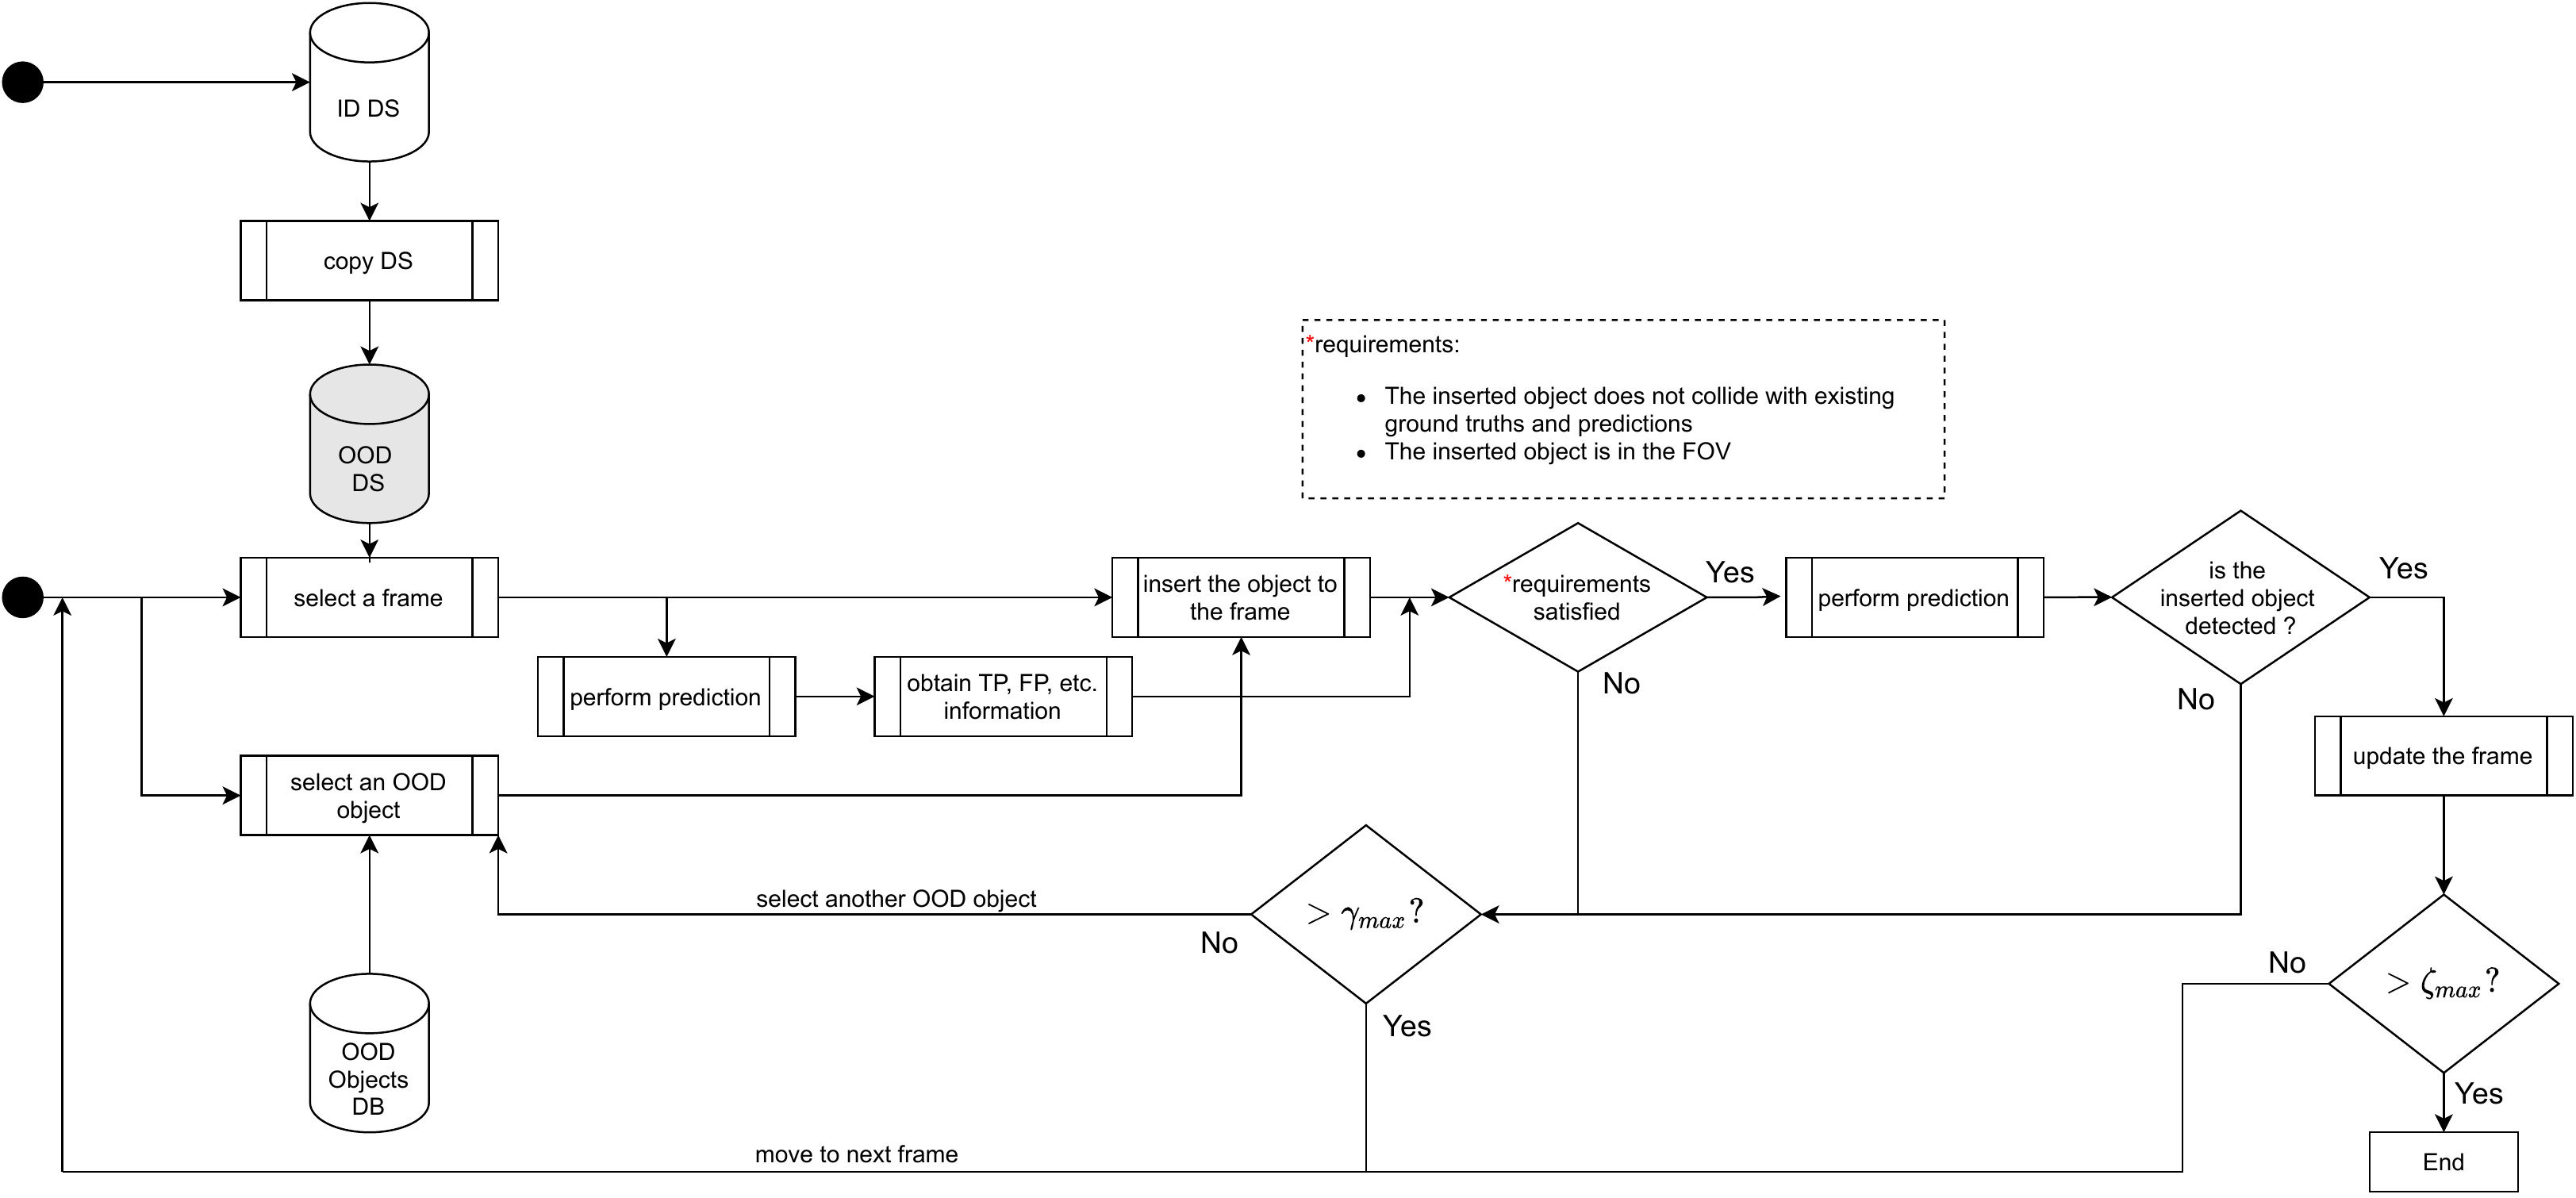}
\end{center}
\caption{
OOD dataset generation diagram
}
\label{fig:ood_gen_diagram}
\end{figure*}

We utilize different sources to gather OOD objects to be inserted into the KITTI
dataset \cite{geiger2013kittidataset}. For synthetic objects, we use the Carla
simulation \cite{dosovitskiy2017carla}. We run LiDAR simulation to obtain the
point cloud of objects at various angles and distances. For real objects, we use
the KITTI ignored objects, the KITTI False Positive (FP) objects, and weird
vehicle objects from the Waymo dataset \cite{waymo}. For Carla objects, we set
the intensity values for the points to the median of the KITTI intensities. For
Waymo objects, we transform the original intensities using $\tanh$ then adjust
the intensity values so that the mean and variance under log scale is the same
as the KITTI intensities under log scale.

% \Cref{fig:ood_objects} shows some examples of the objects selected from
% different sources. 
The KITTI FP objects are background objects classified as Pedestrians. We
manually label and categorize them into classes such as \textit{potted plant,
bike rack, low traffic sign, sidewalk sign}, and \textit{thin sign}.
Furthermore, we verify if KITTI FP objects appear in the KITTI training dataset.
The \Cref{tab:fp-in-training} shows that except bike rack, other KITTI FP
objects do appear relatively frequently in the KITTI training dataset.
Therefore, KITTI FP objects are a good candidate for the type
\textcircled{\small 5} OOD objects.
\begin{table}[H]
\centering
\tiny
\begin{tabular}{c|ccccc}
\toprule
Class &   Bike rack & Sidewalk sign & Traffic sign & Potted plant & Thin sign \\
\midrule
Quantity  & 0 &  625 & 295 & 298 & 60\\
\bottomrule
\end{tabular}
\caption{The number of times that KITTI FP objects appear in the KITTI training dataset}
\label{tab:fp-in-training}
\end{table}
We manually identify objects among the Waymo vehicle class that are not FG in
KITTI, including \textit{motorcycle, scooter, digger, and excavator}. To ease
the annotation procedure, we first cluster all collected vehicles in the Waymo
validation dataset into either a \textit{main} cluster or an \textit{outlier}
cluster using the DBSCAN algorithm and only annotate the vehicles clustered into
the \textit{outlier} cluster. We run four separate DBSCAN clusterings on the
following four sets of features: $\text{PCA}([l, w, h, l/w, l/h, w/h, lw, lh,
wh], \text{ndim}=2)$, $[l,w]$, $[l,h]$, and $[w,h]$, where $l$, $w$, and $h$
correspond to the length, width, and height of the collected vehicle,
respectively. We then define the global outlier cluster as $\{ \text{vehicles }
v | v \text{ is an outlier in at least one clustering} \}$. Next, we manually
collect the vehicles in the global outlier cluster that are likely to be OOD
objects for the KITTI dataset and assign a class label to each collected
out-of-distribution vehicle. Finally, we collect the LiDAR point cloud of each
annotated outlier Waymo vehicle across multiple frames (every ten frames) in the
scene where the vehicle exists.
\begin{table*}
\centering
\tiny
\begin{tabular}{c|c|c|cccc|cccc|c}
\toprule
\multirow{3}{*}{Type} & \multirow{3}{*}{Class} & & \multicolumn{4}{c}{Base model} &  \multicolumn{4}{c}{Contrastive model} &
\\
&  & \# instances &
\# injection & \# detection & \# attempted & \# injected &
\# injection & \# detection & \# attempted & \# injected & 
\# common \\
& & in DB &
failures & failures & frames & objects &
failures & failures & frames & objects & 
OOD \\
\midrule
\multirow{5}{*}{Carla} 
 & ATM          & 10 & 17.51 &  43.52 & 545     & 300    & 16.20 & 40.25 & 489     & 300 & 289.67 \\ %262 & 309 & 298 \\
 & Bench        & 44 & 25.97 &  64.74 & 2342.67 & 289.33 & 22.61 & 55.70 & 1229.67 & 300 & 318.67 \\ %281 & 320 & 355 \\
 & Swing couch  & 25 & 29.37 &  60.96 & 2276.33 & 267.67 & 24.38 & 48.01 & 1631    & 300 & 200.67 \\ % 134 & 299 & 169 \\
 & Trash can 1  &  5 & 18.65 &  49.22 & 638.33  & 300    & 15.43 & 39.92 & 470.67  & 300 & 537.67 \\ % 549 & 542 & 522 \\
 & Trash can 2  &  5 & 4.02  &  9.38  & 304.67  & 300    & 2.39  & 5.40  & 302     & 300 & 582 \\ % 591 & 590 & 565 \\
\midrule
\multirow{4}{*}{KITTI Ignored} 
 & Tram             & 287 & - & - & - & - & - & - & - & - & 73.33 \\ % 67  & 60 & 105 \\
 & Truck            & 606 & - & - & - & - & - & - & - & - & 69.67 \\ % 68  & 72 & 69  \\
 & Person sitting   & 166 & - & - & - & - & - & - & - & - & 105.33 \\ % 106 & 114 & 96 \\
 & Misc             & 636 & - & - & - & - & - & - & - & - & 138 \\ % 139  & 152 & 123 \\
\midrule
\multirow{5}{*}{KITTI FP} 
 & Bike rack        & 11 & 0.71 & 0.04  & 300 & 300 & 0.93 & 0.09 & 300  & 300 & 599 \\ % 598  & 600 & 599 \\
 & Low traffic sign & 10 & 0.33 & 0.016 & 300 & 300 & 0.22 & 0.02 & 300  & 300 & 598.67 \\ % 597  & 599 & 600 \\
 & Sidewalk sign    & 33 & 0.57 & 0.008 & 300 & 300 & 0.37 & 0.02 & 300  & 300 & 599 \\ % 600 & 597 & 600 \\
 & Potted plant     & 9  & 0.89 & 0.03  & 300 & 300 & 0.69 & 0.03 & 300  & 300 & 599.33 \\ % 599 & 600 & 599 \\
 & Thin sign        & 3  & 0.54 & 0.084 & 300 & 300 & 0.36 & 0.06 & 300  & 300 & 598.67 \\ % 599 & 600 & 597 \\
\midrule
\multirow{4}{*}{Waymo}
 & Motorcycle   & 456 & 4.07 &  0.81 & 300    & 300 & 3.80  & 0.74 & 300    & 300 & 512 \\ % 519  & 502 & 515 \\
 & Scooter      & 80  & 9.68 &  1.39 & 300    & 300 & 8.18  & 1.01 & 300    & 300 & 385.67 \\ % 437 & 338 & 382 \\
 & Digger       & 49  & 4.57 &  1.03 & 300    & 300 & 4.48  & 1.00 & 300    & 300 & 585.67 \\ %588 & 583 & 586 \\
 &Excavator    & 44  & 13.35 &  3.04 & 302.33 & 300 & 11.67 & 2.65 & 300.33 & 300 & 564.33 \\ % 569  & 549 & 575 \\
\bottomrule
\end{tabular}
\caption{Statistics for OOD objects. In total, we generate six datasets, one for each model/seed combination. The injection statistics (\# injection failures, \# detection failures, \# attempted frames, \# injected objects) and \# common OOD are averaged over three seeds. }
\label{tab:object_statistics}
\end{table*}

%%%%%%%Base
% Atm
% [ 17.51  43.52 545.        ]
% Bench01
% [  25.97   64.74 2342.66]
% SwingCouch
% [  29.37   60.96 2276.33]
% TrashCan01
% [ 18.65  49.22 638.33]
% TrashCan02
% [  4.02    9.38 304.66]

% bike_rack
% [  0.71   0.04 300.   ]
% low_traffic_sign
% [  0.33   0.016 300.   ]
% sidewalk_sign
% [  0.57    0.01 300.   ]
% potted_plant
% [  0.89   0.03 300.   ]
% thin_sign
% [  0.54    0.08 300.   ]

% motorcycle
% [  4.07   0.81 300.        ]
% scooter
% [  9.68   1.39 300.        ]
% digger
% [  4.57   1.03 300.        ]
% excavator
% [ 13.35   3.04 302.33]

%%%%%%%%Contrastive
% Atm
% [ 16.20 40.25  489.0        ]
% Bench01
% [ 22.61 55.70 1229.66]
% SwingCouch
% [ 24.38 48.01 1631.0        ]
% TrashCan01
% [ 15.43 39.92 470.66]
% TrashCan02
% [  2.39 5.40 302.0        ]

% bike rack
% [  0.93   0.09  300.   ]
% low_traffic_sign
% [  0.22   0.02 300.   ]
% sidewalk_sign
% [  0.37   0.02  300.   ]
% potted_plant
% [  0.69   0.03 300.   ]
% thin_sign
% [  0.36   0.06 300.   ]

% motorcycle
% [  3.80 0.74 300.        ]
% scooter
% [  8.18 1.01 300.        ]
% digger
% [  4.48 1.0 300.        ]
% excavator
% [ 11.67 2.65 300.33]

In \Cref{tab:object_statistics}, we list the number of objects per class from
each OOD database that we select to create OOD datasets. We select these classes
because, based on our experiment, they are likely to be misclassified as
foreground objects when we insert them into the KITTI validation dataset.
For each class, we insert 300 objects into an OOD dataset. The number of
attempted frames is the number of frames the algorithm must go through to insert
300 objects. In each frame, the maximum number of trials is 100. If the number
of trials exceeds the maximum number of trials, we abandon the frame and move on
to the next frame. \Cref{tab:object_statistics} also shows the statistics of
inserting objects from each database to create OOD datasets. Injection failures
and detection failures are the numbers of failed trials averaged over the number
of attempted frames. The higher injection failures, the higher chance that an
object overlaps with existing objects in a frame. The higher the detection
failures, the lower likelihood that an object is detected when we insert it into
a frame. For example, in Carla OOD datasets, bench and swing couch have high
injection failures because they are large objects. Thus, they easily overlap
with existing objects in a frame. These objects also have high detection
failures because a model cannot easily detect them. Furthermore, by comparing
the statistics among datasets, we can conclude that it is easier to insert Waymo
and KITTI FP objects than to insert Carla objects. It makes sense because LiDAR
sensors in both Waymo and KITTI datasets have a similar specification. In
contrast, the Carla objects are synthetic data from a simulation. In addition,
it is easier to insert Carla objects using the contrastive model than the base
model. The observation is opposite for the Waymo and KITTI FP objects.
